# Supplementary material for: What's in a Latent? Leveraging Diffusion Latent Space for Domain Generalization
Source: arXiv:2503.06698 source file (2025-04-28)
Supplement: Supplementary file 1 [file nmi_class_domain.tex]

\begin{figure}[!h]
    \centering
    % First row: PACS
    \begin{minipage}{0.7\linewidth}
        \centering
        \includegraphics[width=\linewidth]{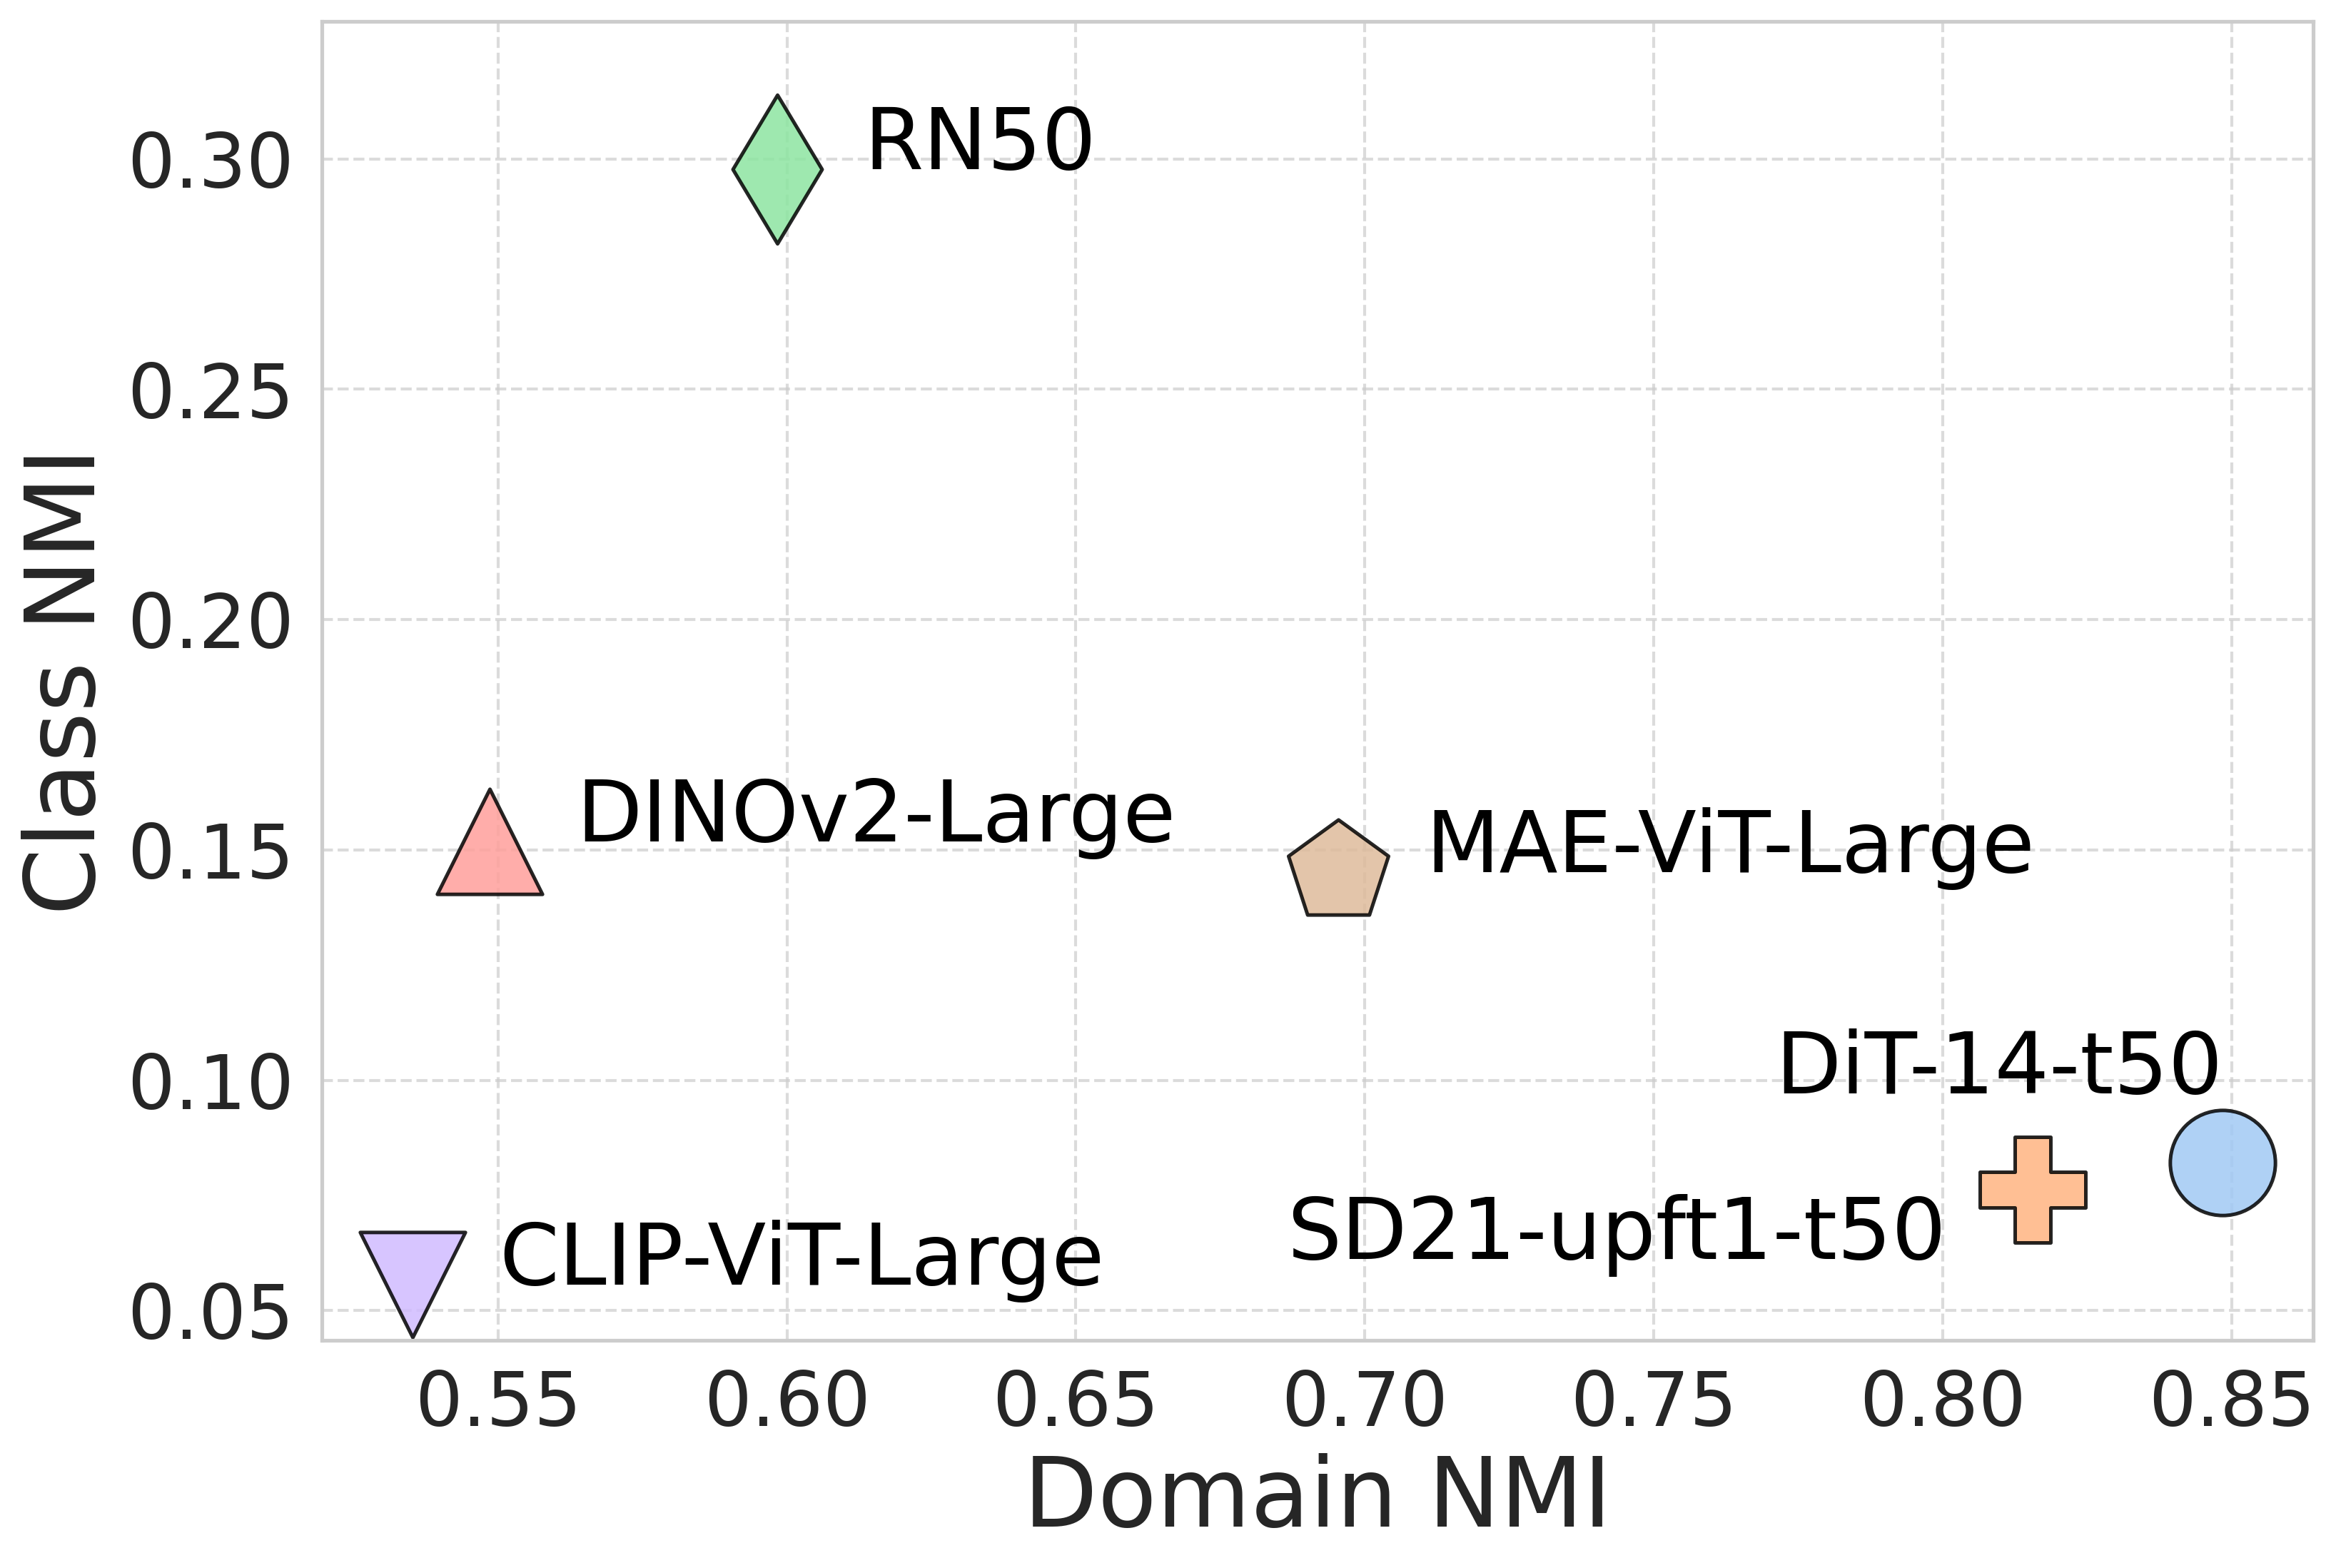}
        \vspace{-1.8em} % Reduce spacing before subfigure caption
        \caption*{\scriptsize (a) PACS}
        \label{fig:pacs_class_domain_nmi}
    \end{minipage}
    
    \vspace{0.5em} % Adjust vertical spacing between rows

    % Second row: VLCS
    \begin{minipage}{0.7\linewidth}
        \centering
        \includegraphics[width=\linewidth]{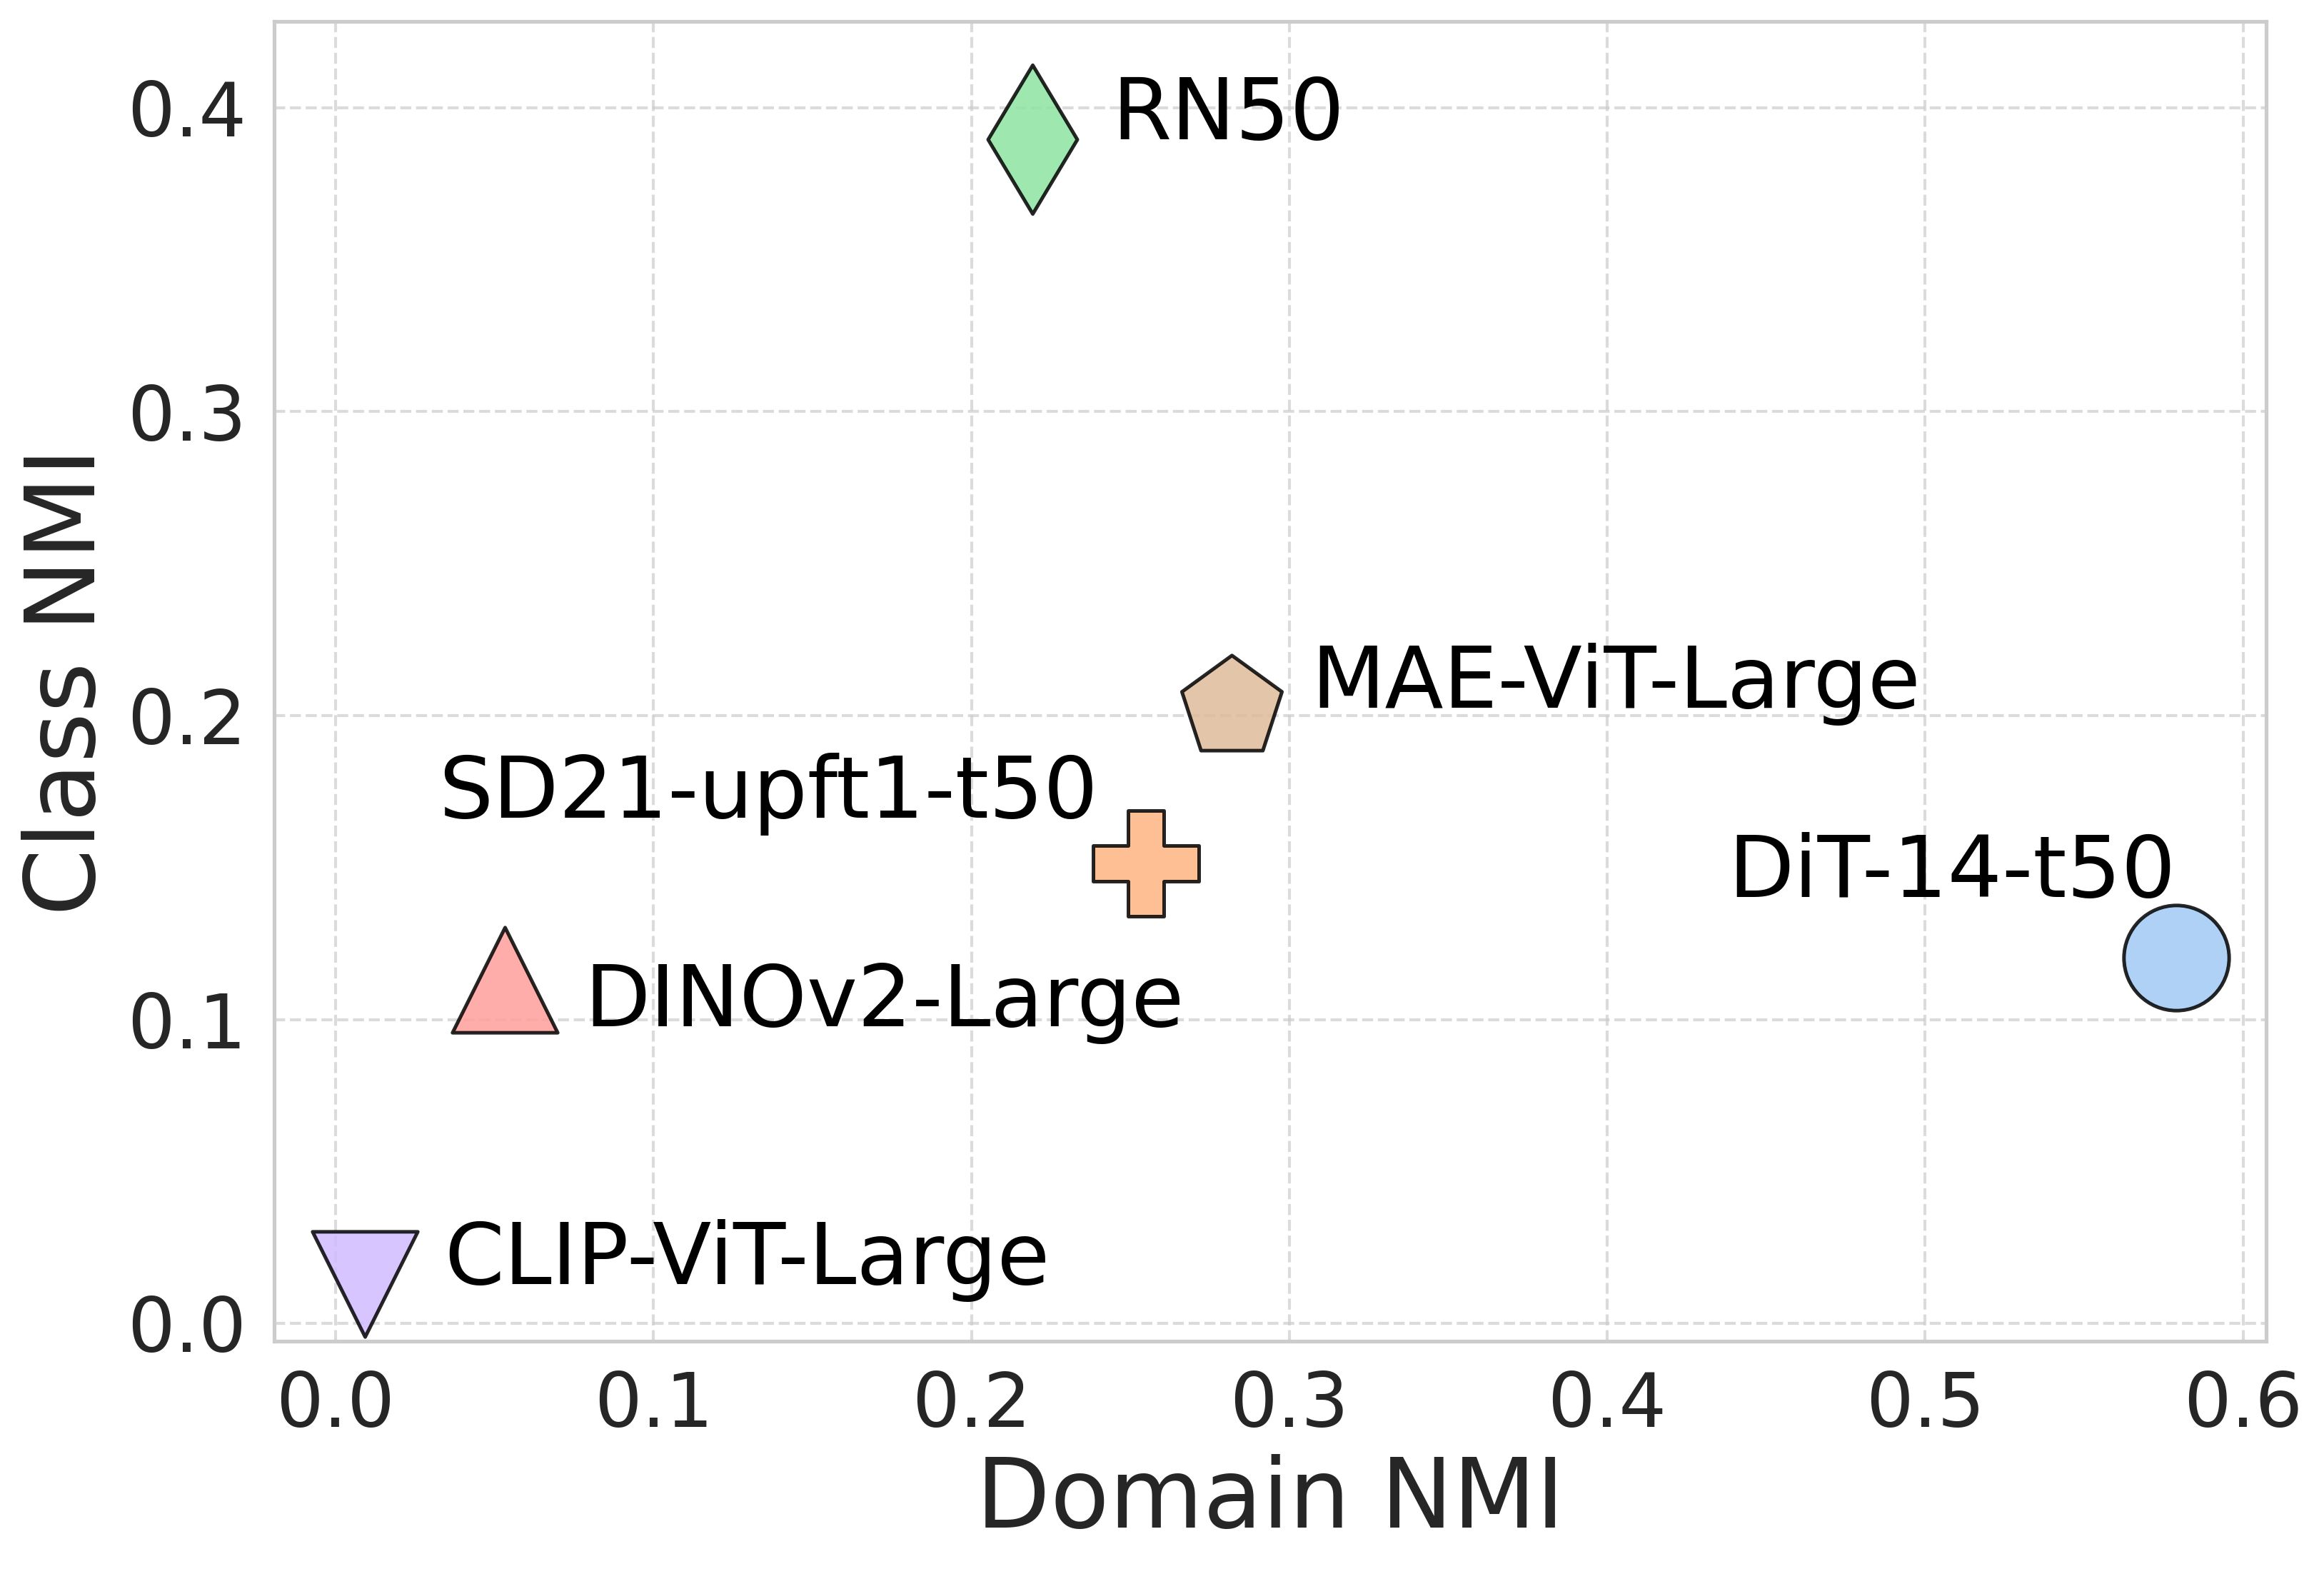}
        \vspace{-1.8em} % Reduce spacing before subfigure caption
        \caption*{\scriptsize (b) VLCS}
        \label{fig:vlcs_class_domain_nmi}
    \end{minipage}
    
    \vspace{-0.8em} % Reduce spacing before main caption
    \caption{\footnotesize \textbf{Class-Domain NMI visualizations for PACS and VLCS datasets for the $\bPsi$ feature space.} Diffusion-based models (SD-2.1, DiT) exhibit the highest Domain NMI scores while maintaining relatively low Class NMI scores, suggesting that their latent spaces are well-suited for capturing domain-specific, class-invariant structures. Note that $\bPsi$ aims at capturing domain-specific variances for {\algoname}. Also, note that the extent of domain separation in $\bPsi$ is dependent on the nature of domain shifts (as seen in the relative drop of Domain NMI score of SD-2.1 for VLCS), as discussed in Sec~\ref{sec:pretrain_obj}. \xavier{can remove for space, if needed.} \deepti{move this to appendix for now}}
    \label{fig:class_domain_nmi}
\end{figure}
