# Supplementary material for: What's in a Latent? Leveraging Diffusion Latent Space for Domain Generalization
Source: arXiv:2503.06698 source file (2025-04-28)
Supplement: Supplementary file 2 [file adaptivity_gap.tex]

\begin{figure}[!h]
    \centering
    {\includegraphics[width=0.8\linewidth]{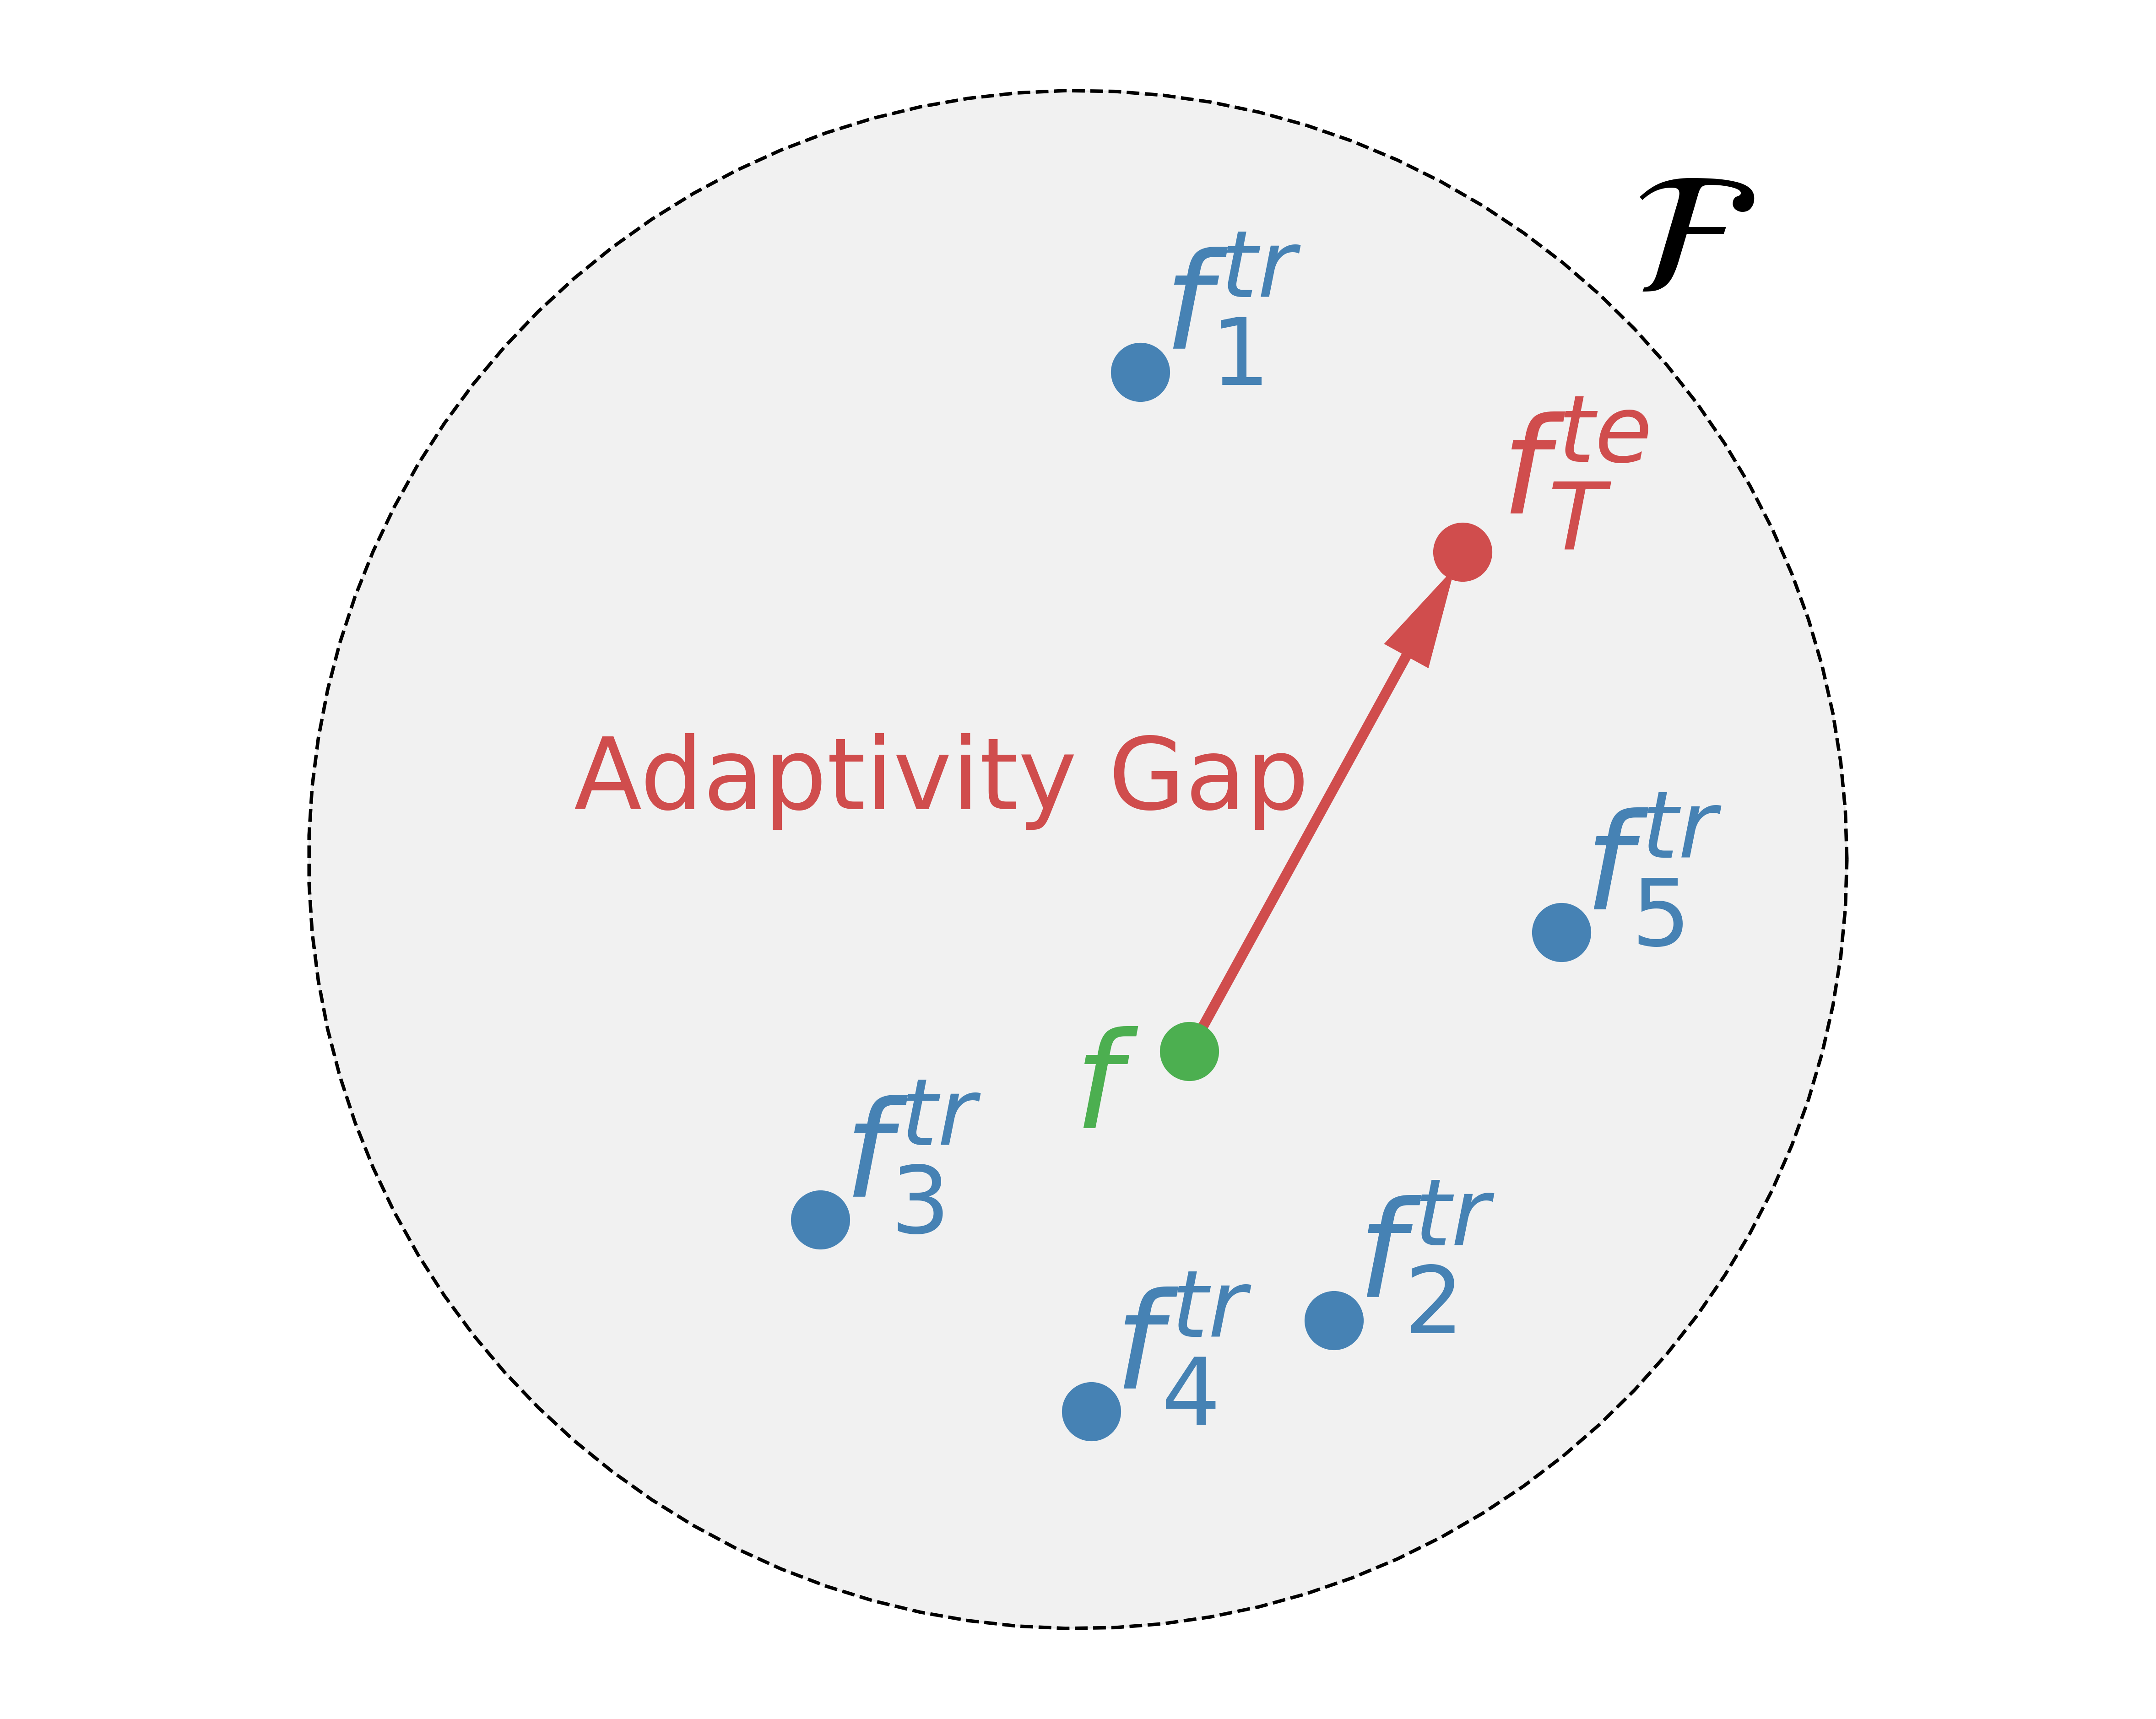}}\hfill \\ 
    \caption{\footnotesize{\textbf{A visual representation of the adaptivity gap}~\cite{Dubey2021AdaptiveMF} \textbf{in learning a generalizable classifier in a multi-domain setting.} The optimal universal classifier \(f \in \mathcal{F}\), trained on all training domains, may differ significantly from the optimal classifier for the unseen test domain \(d^{te}\), highlighting the need for methods that adapt to domain-specific variations.}}
    \label{fig:adaptive_gap}
    % \vspace{-0.05in}
    % k-SAE visualization at \texttt{up\_ft1} for $t=25$ on Oxford-Pets dataset.
\end{figure}
