# Supplementary material for: What's in a Latent? Leveraging Diffusion Latent Space for Domain Generalization
Source: arXiv:2503.06698 source file (2025-04-28)
Supplement: Supplementary file 3 [file pacs_dit_feat_space.tex]

\begin{figure}[!h]
    \centering
    {\includegraphics[width=1\linewidth]{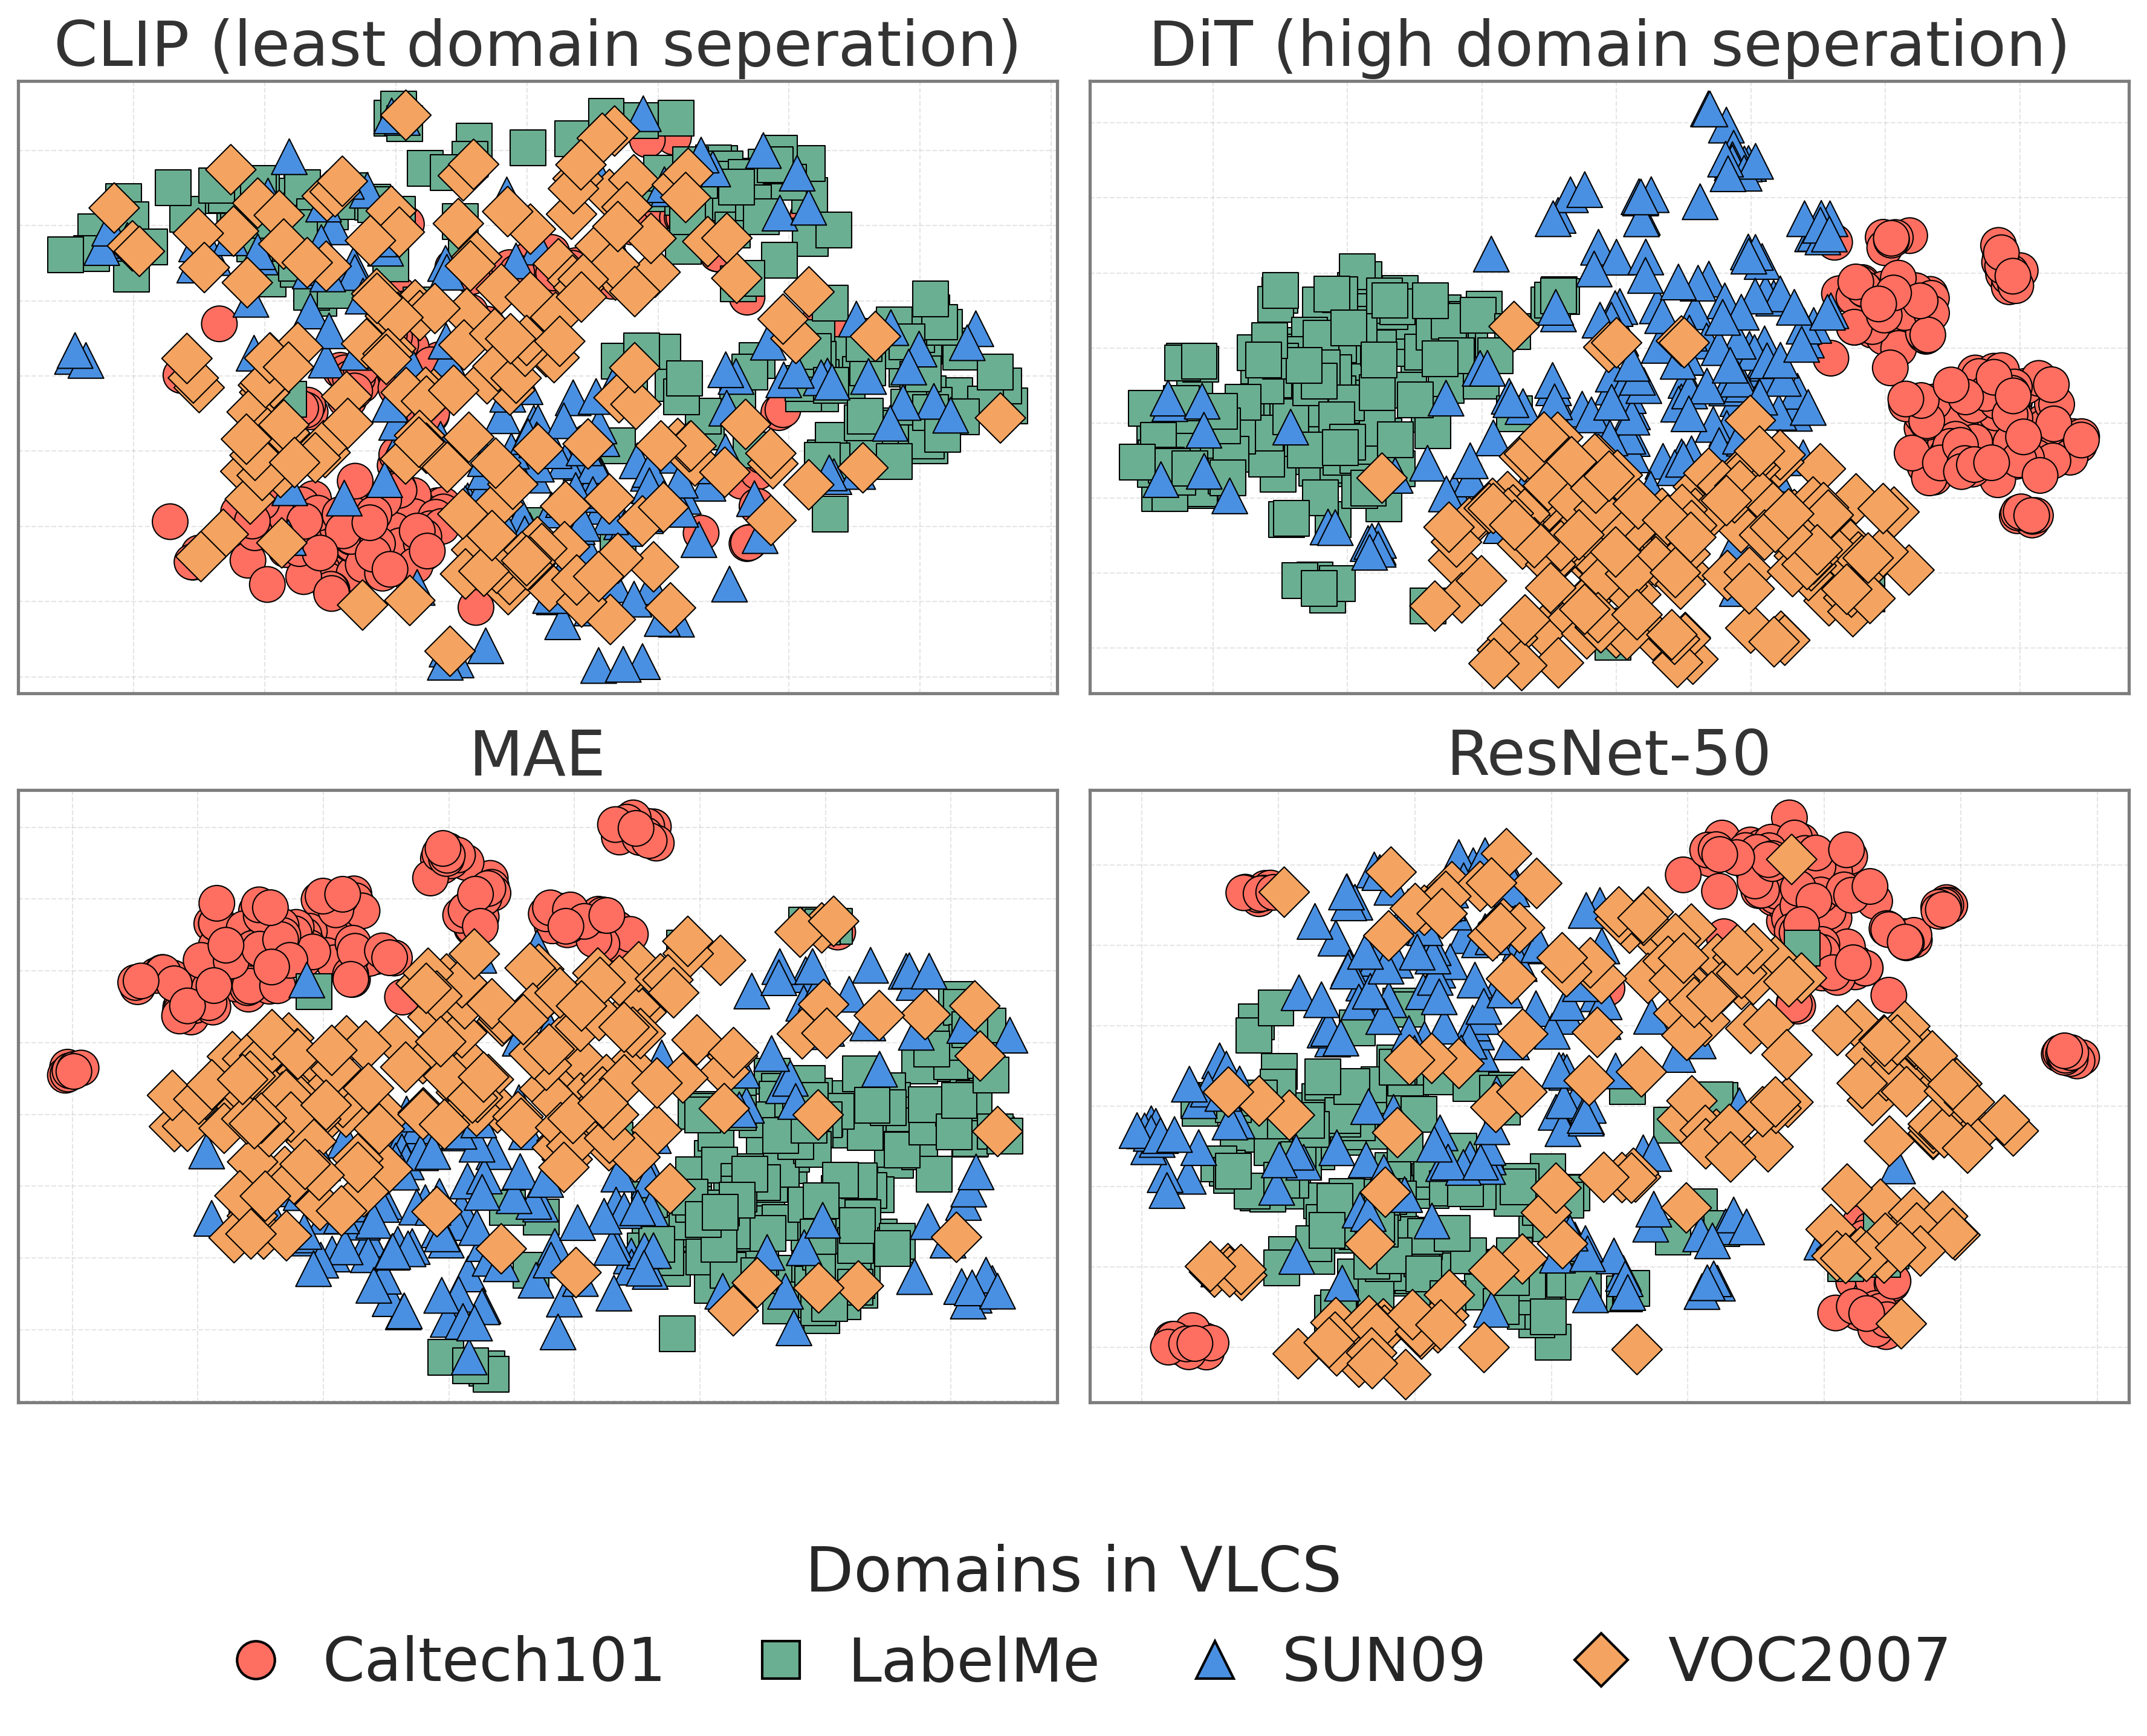}}\hfill \\ 
    \caption{\footnotesize{\textbf{k-sparse autoencoders (k-SAE)} trained on complex visual features help identify monosemantic visual properties represented within black-box diffusion models. We show sample k-SAE neurons and top-4 images that yield highest activations when the k-SAE is trained on intermediate diffusion layer's features on \oxford~\cite{oxford} dataset. Note how these features encapsulate distinct fine-grained information about different breeds like \textit{Keeshond} and \textit{Samoyed}. Best viewed in color.
    } }\label{fig:main}
    % \vspace{-0.05in}
    % k-SAE visualization at \texttt{up\_ft1} for $t=25$ on Oxford-Pets dataset.
\end{figure}
