# Supplementary material for: What's in a Latent? Leveraging Diffusion Latent Space for Domain Generalization
Source: arXiv:2503.06698 source file (2025-04-28)
Supplement: Supplementary file 4 [file psuedo_image.tex]

\begin{figure}[!h]
    \centering
    {\includegraphics[width=0.99\linewidth]{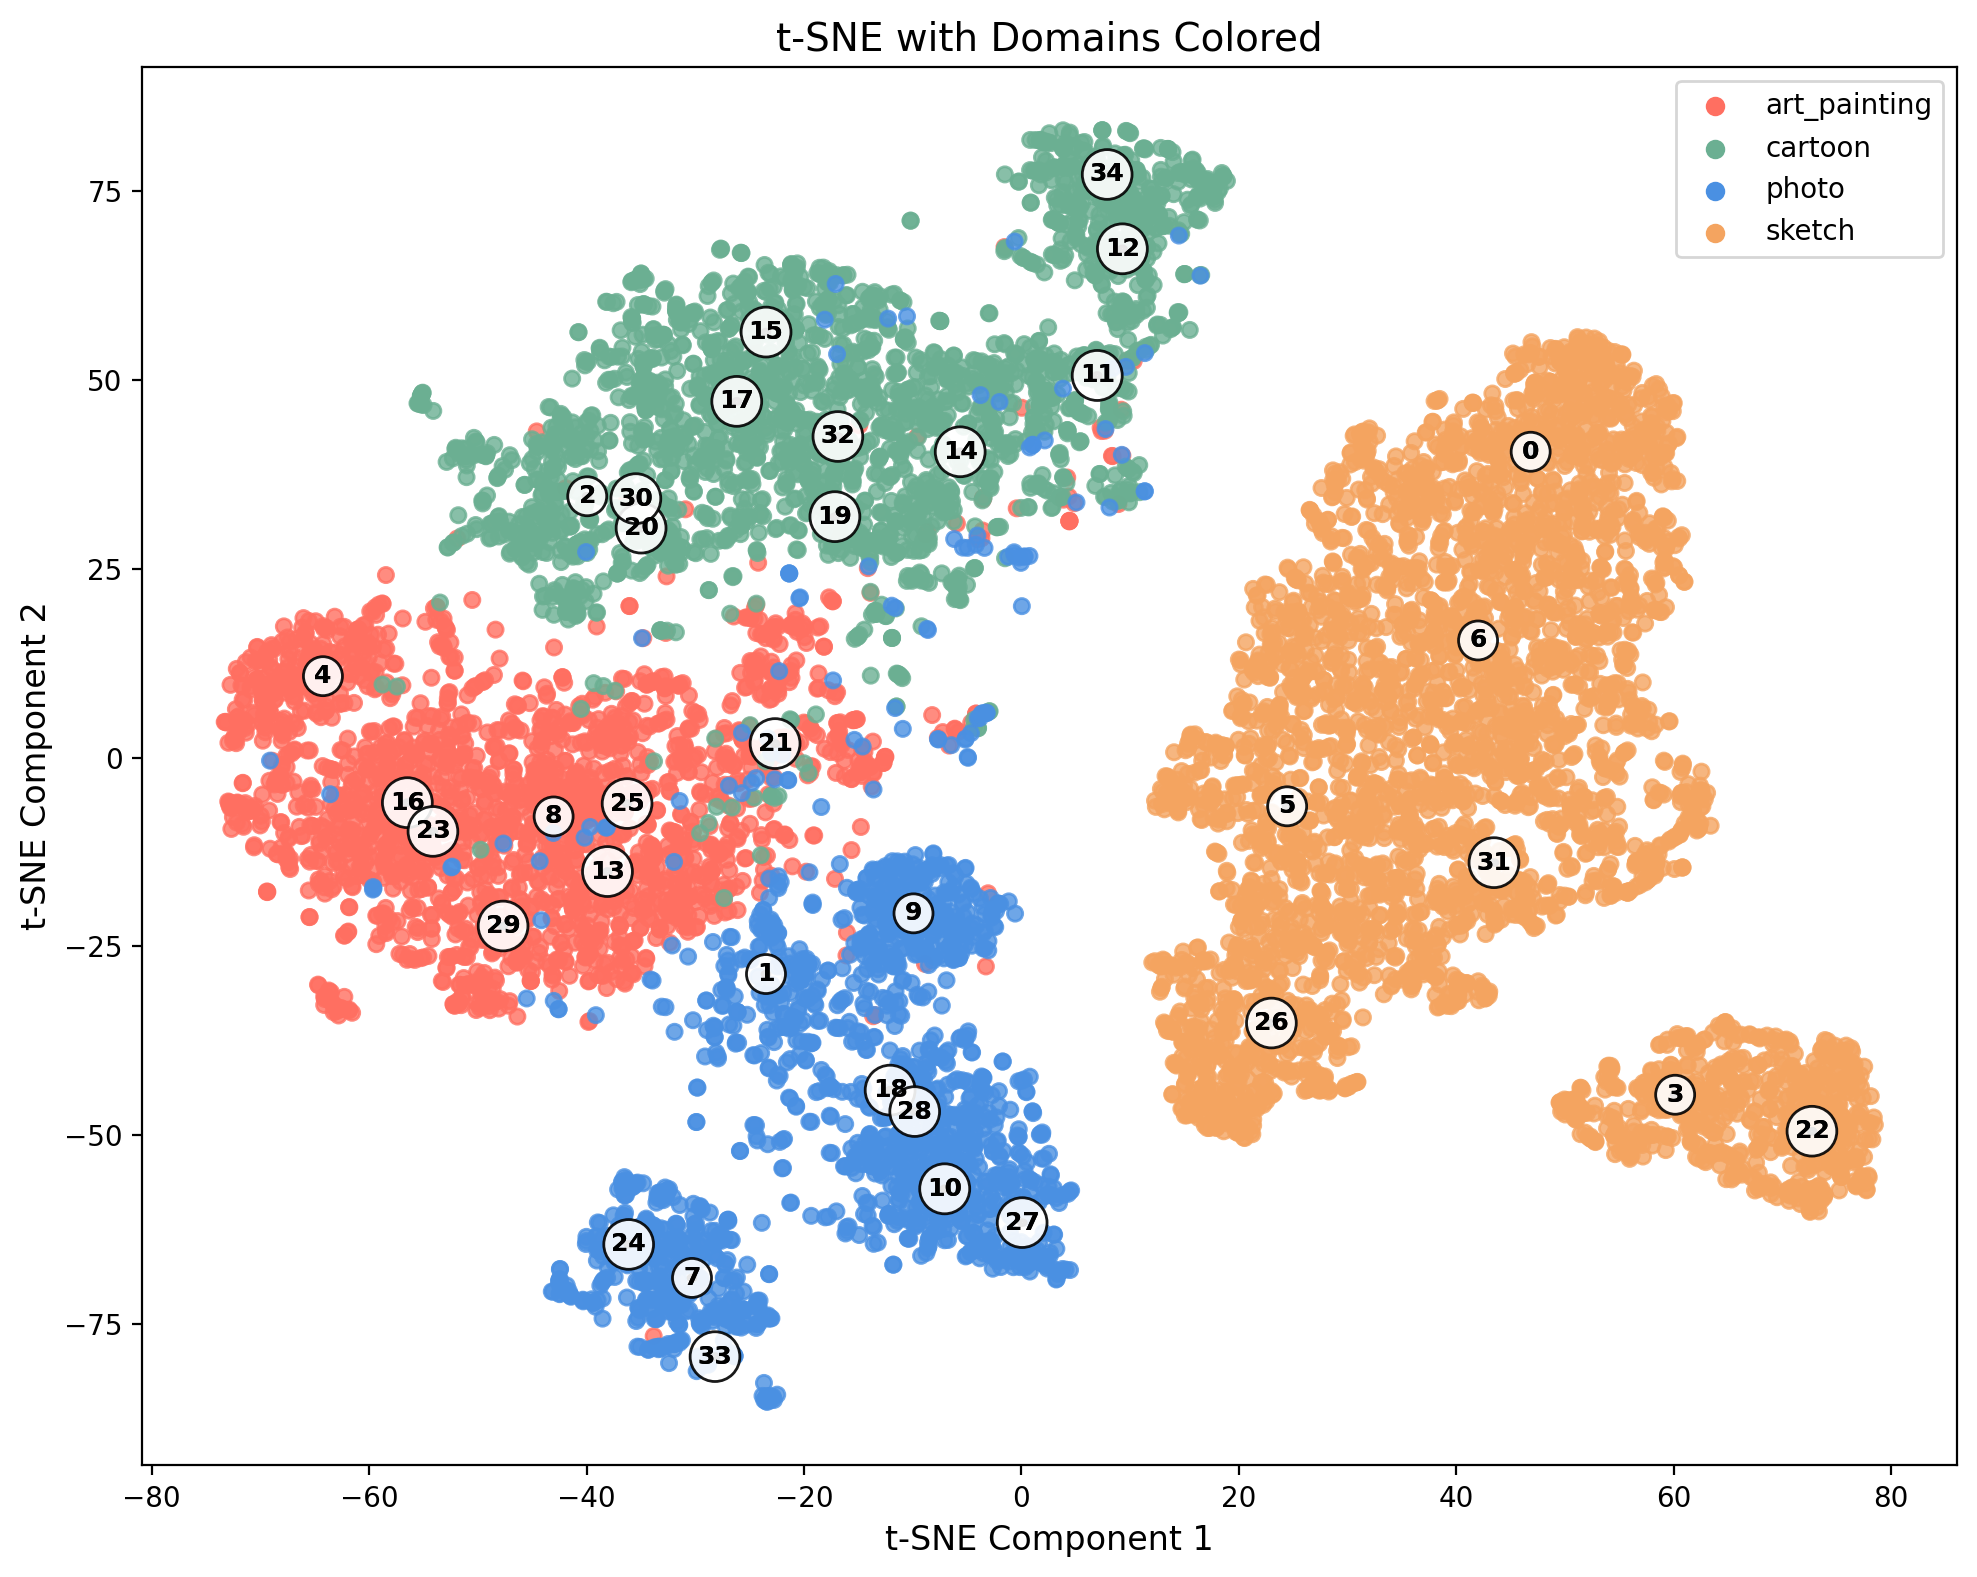}}\hfill \\ 
    \caption{\footnotesize{\textbf{A visual representations of the pseudo-domain clusters}}}
    \label{fig:pseudo_image}
    % \vspace{-0.05in}
    % k-SAE visualization at \texttt{up\_ft1} for $t=25$ on Oxford-Pets dataset.
\end{figure}
